# Supplementary material for: Biorthogonal Bulk-Boundary Correspondence in Non-Hermitian Systems
Source: arXiv:1805.06492 ancillary file (2018-07-15)
Supplement: Supplementary file 1 [file Non-Hermitian_models_supplementary_material_1806.pdf]

# Supplementary Material for Biorthogonal Bulk-Boundary Correspondence in Non-Hermitian Systems

Flore K. Kunst[1], Elisabet Edvardsson[1], Jan Carl Budich[2], and Emil J. Bergholtz[1]
[1] *Department of Physics, Stockholm University, AlbaNova University Center, 106 91 Stockholm, Sweden*
[2] *Institute of Theoretical Physics, Technische Universität Dresden, 01062 Dresden, Germany*
(Dated: June 18, 2018)

In this supplementary material, we provide additional quantitative and technical details on the results discussed in the main text. Specifically, we explicate that the biorthogonal polarization $P$ defined in Eq. (7) is quantized in generic lattice models, we provide more details and additional plots on the phase diagram for the non-Hermitian Rice-Mele Chern insulator model shown in Fig. 2 in the main text. Furthermore, we provide quantitative details on the crossover between periodic and open boundary conditions as well as the two-domain ring geometry discussed in the main text for the non-Hermitian SSH chain.

## QUANTIZED BIORTHOGONAL POLARIZATION

Here we provide details on the biorthogonal polarization $P$ defined in Eq. (7) in the main text. In particular, we discuss for an explicit non-exactly solvable example that the biorthogonal polarization jumps between the values zero and one for generic boundary modes, irrespective of whether the number of sites is even or odd. By making use of the exact solutions in Eqs. (3) and (4) in the main text, which are relevant both for models with a broken unit cell and with unbroken unit cells, it is straightforward to show that $P = 1$ ($P = 0$) when $|r_L^* r_R| < 1$ ($|r_L^* r_R| > 1$), which in the case of a termination with a broken unit cell corresponds to a boundary mode localized to the unit cell $n = 1$ ($n = N$) and in the case of unbroken unit cells to the presence (absence) of boundary modes.

This result for the biorthogonal polarization also holds for boundary modes of a more general form that are not captured by our exact solutions. Using the biorthogonal normalization condition, we find

$$\begin{aligned} 0 &= 1 - \lim_{N\to\infty} \left\langle \Psi_L \left| \sum_{n=1}^{N} \Pi_n \right| \Psi_R \right\rangle = 1 - \lim_{N\to\infty} \left\langle \Psi_L \left| \frac{\sum_{n=1}^{N} [n + (N-n)]\Pi_n}{N} \right| \Psi_R \right\rangle \\ &= P - \lim_{N\to\infty} \left\langle \Psi_L \left| \frac{\sum_{n=1}^{N} (N-n)\Pi_n}{N} \right| \Psi_R \right\rangle , \end{aligned}$$

with the biorthogonal polarization $P$ as defined in Eq. (7) in the main text. If the boundary mode described by $|\psi_R\rangle, |\psi_L\rangle$ is localized to a unit cell with small $n$, we trivially find $P = 1$. However, if the mode is localized close to site $N$, it is straightforward to find that $P = 0$. Hence, for a general boundary mode $P$ jumps between 0 and 1.

To quantitatively corroborate that the biorthogonal polarization $P$ is the relevant predictive quantity beyond exactly-solvable models, we present numerical data for the Haldane model [1] with non-Hermitian hopping terms that realizes a Chern-insulating phase on the honeycomb lattice and where the edge states cannot be readily found exactly due to next-nearest-neighbor hopping terms. The Bloch Hamiltonian reads $H = \Psi^\dagger \mathcal{H}_{\mathbf{k}} \Psi$ with $\Psi^\dagger = (c^\dagger_{A,\mathbf{k}}, c^\dagger_{B,\mathbf{k}})$, $\mathcal{H}_{\mathbf{k}} = \mathbf{d}(\mathbf{k}) \cdot \boldsymbol{\sigma}$ and

$$d_x(\mathbf{k}) = t_1 \sum_{i=1}^{3} \cos(k_i) - i\frac{\gamma}{2} \sum_{i=1}^{2} \sin(k_i), \qquad d_y(\mathbf{k}) = -t_1 \sum_{i=1}^{3} \sin(k_i) - i\frac{\gamma}{2} \sum_{i=1}^{2} \cos(k_i), \qquad d_z(\mathbf{k}) = -t_2 \sum_{i=1}^{3} \sin(k_i'),$$

where $A$ and $B$ are the sublattices, $t_1$ ($t_2$) is the (next-)nearest-neighbor hopping parameter, $k_i \equiv \mathbf{k} \cdot \boldsymbol{\delta}_i$, $k_i' \equiv \mathbf{k} \cdot \boldsymbol{\delta}_i'$, and $\boldsymbol{\delta}_i$ ($\boldsymbol{\delta}_i'$) are the (next-)nearest-neighbor vectors; $\boldsymbol{\delta}_1 = (1, 1/\sqrt{3})/2$, $\boldsymbol{\delta}_2 = (-1, 1/\sqrt{3})/2$, $\boldsymbol{\delta}_3 = -(0, 1/\sqrt{3})$, $\boldsymbol{\delta}_1' = (1, \sqrt{3})/2$, $\boldsymbol{\delta}_2' = (1, -\sqrt{3})/2$ and $\boldsymbol{\delta}_3' = -(1, 0)$. Taking open boundary conditions in $y$, we plot the spectrum for the cylinder configuration with zigzag edges on both sides in Fig. 1. Due to the non-degeneracy of the chiral bands, the biorthogonal polarization can now be defined directly for a model with un-broken unit cells (even number of sites) so as to provide information on the localization of the chiral modes. In Fig. 1(a), we show the spectrum for a model with no broken unit cells and find two chiral modes inside the gap of which the right (in red) and left (in cyan) mover have a polarization of $P = 1$ and $P = 0$, respectively, such that they are localized to the respective unit cells $n = 1$ and $n = N$. In Fig. 1(b), we add a potential to the $B$ sublattice in unit cell $n = N$ by which we effectively introduce

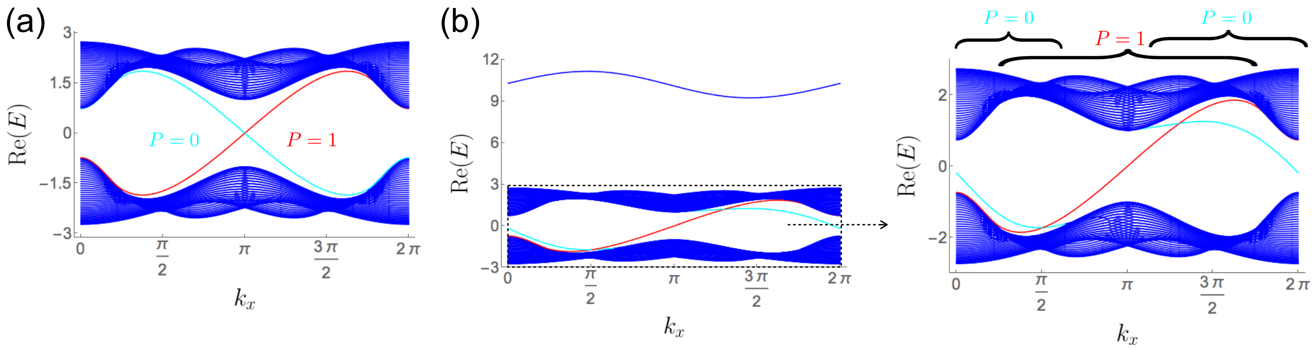


FIG. 1: The real part of the energy spectrum for the Haldane model on a honeycomb lattice with zigzag edges with $N = 46$ sites, $t = t_2 = \gamma = 1$ and an edge potential $V = 10$ on the $B$ sites in the unit cell $n = N$ in (b). The biorthogonal polarization $P = 1$ ($P = 0$) for the right (left) mover in red (cyan).

a domain wall and the system behaves as if it has a broken unit cell on the edge $n = N$. Indeed, chiral modes exist for all $k_x$ and we find a polarization $P = 1$ ($P = 0$) for the right (left) mover shown in red (cyan) in agreement with our previous statements.

## SU-SCHRIEFFER-HEEGER MODEL IN THE HERMITIAN LIMIT

For clarity, we here include the energy spectrum for the non-Hermitian SSH model, whose Bloch Hamiltonian is given in Eq. (8) in the main text, and compare the Hermitian limit, i.e., $\gamma \to 0$, with the non-Hermitian case. In this limit, the ordinary bulk-boundary correspondence is retrieved as shown in Fig. 2(a), where we see that the gap closing in the periodic case (black dotted lines) corresponds to the gap closings in the open system (orange lines). By turning on $\gamma$, Figs. 2(b) and 2(c), we see that the spectra are smoothly connected and the open system (in blue) behaves qualitatively different from the periodic system (gray).

## PHASE DIAGRAM OF THE TWO-DIMENSIONAL RICE-MELE MODEL

Here we provide additional details on the phase diagram of the Rice-Mele model given in Fig. 2(b) in the main text. According to the condition in Eq. (5) in the main text, the chiral modes of the Rice-Mele model attach to the bulk bands when Eq. (11) in the main text is satisfied, which we repeat here for clarity

$$\cos(k_x) = \frac{\gamma^2}{16t_1\delta}, \pm\sqrt{\frac{\gamma^2/8 - t_1^2}{\delta^2}}. \tag{1}$$

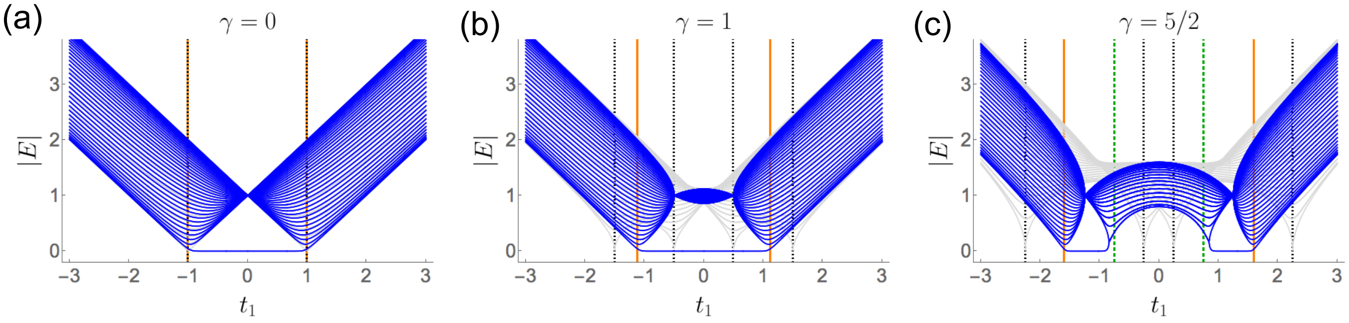


FIG. 2: The absolute value of the eigenvalues of the open SSH model with $t_1 = t_2 = 1$ in the (a) Hermitian limit, i.e., $\gamma = 0$, and in the non-Hermitian case with (b) $\gamma = 1$ and (c) $\gamma = 5/2$. The blue (gray) lines correspond to the spectrum of the open (periodic) system. The black dotted vertical lines correspond to the gap closings in the periodic spectrum and the orange (dark green dashed) vertical lines correspond to those points where $r_L^* r_R = 1$ ($r_L^* r_R = -1$).

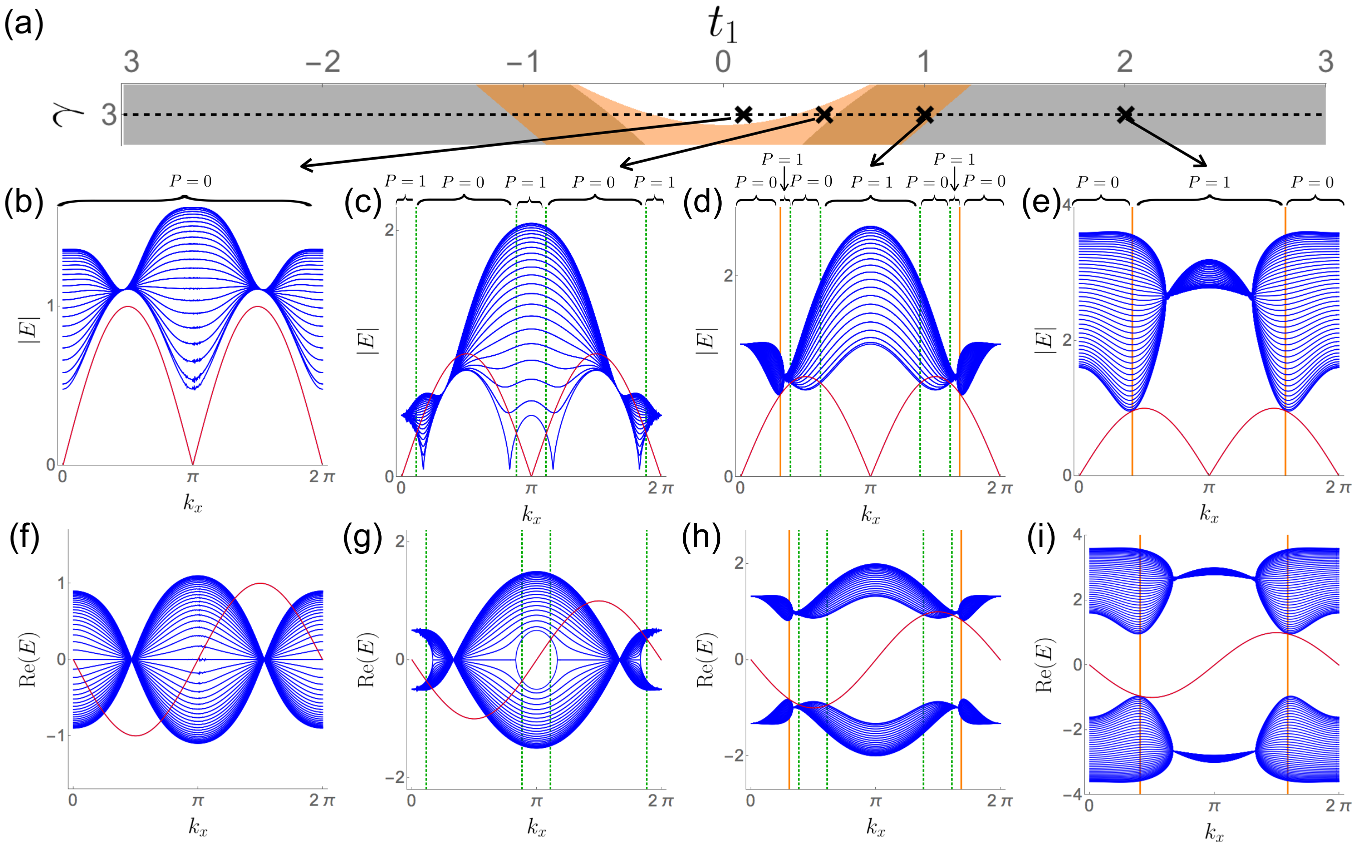


FIG. 3: (a) Zoom in of the bulk phase diagram at $\Delta = \delta = 1$. We plot the (b)-(e) absolute value and (f)-(i) real part of the energy for a system with $N = 46$ with a broken unit cell at $n = 46$, and the parameter values indicated by the crosses in (a); $\gamma = 3$, and (b) and (f) $t_1 = 0.1$, (c) and (g) $t_1 = 0.5$, (d) and (h) $t_1 = 1$, and (e) and (i) $t_1 = 2$ for which 0, 4, 6 and 2 solutions to Eq. (1) exist, respectively. The chiral mode is shown in red and the orange (dark green dashed) vertical lines correspond to those points where $r_L^* r_R = 1$ ($r_L^* r_R = -1$).

We thus find two solutions for $k_x$ when $\gamma^2/(16t_1\delta) \leq 1$ and four solutions when $0 \leq (\gamma^2/8 - t_1^2)/\delta^2 \leq 1$, such that we either have 0, 2, 4 or 6 solutions for $k_x$ depending on the parameter values. A zoom in of the phase diagram is shown in Fig. 3(a), and in Figs. 3(b)-(e) and Figs. 3(f)-(i) we show the absolute value and real part of the energy spectrum of the Rice-Mele model with open boundary conditions for the four different phases indicated by crosses in Fig. 3(a). First of all, we notice that the chiral band only attaches to conductance and valance bands when the number of solutions is non-zero; indeed no solutions exist for the spectra in Figs. 3(b) and (f), while solutions do exist for the parameters chosen in Figs. 3(c)-(e) and (g)-(i). Secondly, going from the phase with no solutions (cf. Figs. 3(b) and (f)) to a phase with four solutions (cf. Figs. 3(c) and (g)) is accompanied by bulk-gap closings, which persist for the entire phase with four solutions. The gap opens again when transitioning to the phase with six solutions (cf. Figs. 3(d) and (h)) and remains open when entering the phase with two solutions (cf. Figs. 3(e) and (i)). In fact, transitioning from the phase with six solutions to a phase with two solutions and vice versa is simply accomplished by a continuous transformation of the bulk bands only. Moreover, when only four solutions exist, they predict where the chiral mode attaches to the bulk after the band has crossed through the bulk gap. The chiral mode also detaches from the bulk above (below) the conduction (valence) bands (cf. Figs. 3(c) and (g)), which is not captured by our predictions. We note, however, that when this happens, the band is not protected by the bulk gap and can be pushed into the bulk bands.

## CROSSOVER PERIODICITY

Here we provide additional quantitative data on how strongly the bulk spectrum of the open, non-Hermitian SSH chain, whose Bloch Hamiltonian is given in Eq. (8) in the main text, is strongly affected by the introduction of

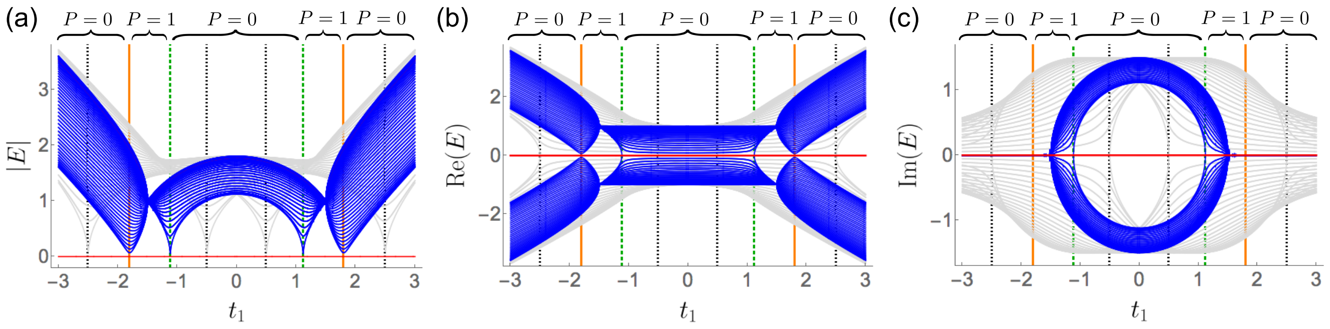


FIG. 4: (a) The absolute value, (b) real and (c) imaginary part of the energy spectrum of the non-Hermitian SSH model in blue as a function of $t_1$ with $t_2 = 1$ and $\gamma = 3$ for $N = 46$ with the last unit cell $n = 46$ broken and the zero mode in red. The gray spectrum originates from the Bloch Hamiltonian with $k = 2\pi n/(2N)$ with $n = 0, 1, .., 2N-1$ and $N = 46$ in all the panels. The orange (dark green dashed) vertical lines correspond to those value of $t_1$ where $r_L^* r_R = 1$ ($r_L^* r_R = -1$) and the gray dotted-dashed lines correspond to the EPs of the periodic Bloch Hamiltonian. The value of the biorthogonal polarization $P$ for the zero mode is indicated at the top of each plot.

weak periodicity. This weak periodicity is established by coupling the ends of the open chain with a term $\Gamma$ similar to the procedure in Ref. 2, such that the Hamiltonian for an *odd* number of sites reads $H = \Psi^\dagger \mathcal{H} \Psi$ with $\Psi^\dagger = (c_{A,1}^\dagger, c_{B,1}^\dagger, c_{A,2}^\dagger, c_{B,2}^\dagger, \ldots, c_{A,N}^\dagger, c_{B,N}^\dagger)$, where $c_{A(B),n}^\dagger$ creates an electron on sublattice $A$ ($B$) in unit cell $n$, and

$$\mathcal{H} = \begin{pmatrix} 0 & t_1 + \frac{\gamma}{2} & 0 & 0 & \cdots & \Gamma t_2 \\ t_1 - \frac{\gamma}{2} & 0 & t_2 & 0 & \cdots & 0 \\ 0 & t_2 & 0 & t_1 + \frac{\gamma}{2} & \cdots & 0 \\ 0 & 0 & t_1 - \frac{\gamma}{2} & 0 & \cdots & 0 \\ \vdots & \vdots & \vdots & \vdots & \ddots & t_1 + \frac{\gamma}{2} \\ \Gamma t_2 & 0 & 0 & 0 & t_1 - \frac{\gamma}{2} & 0 \end{pmatrix}, \tag{2}$$

such that the chain is open (periodic) when $\Gamma = 0$ ($\Gamma = 1$). The band spectrum for this Hamiltonian with $\Gamma = 0$ is shown in Fig. 4, and one can see that there is an exact, non-degenerate zero mode for all $t_1$. In this case, the wave functions in Eqs. (3) and (4) in the main text are exact solutions, and the zero mode is localized to the right (left) end of the chain when the biorthogonal polarization $P = 1$ ($P = 0$). We now study the effect of turning on $\Gamma$ in this model, where the advantage of studying the chain with an odd number of sites lies in the fact that it has an exact zero mode, such that its behavior is straightforwardly quantified. We follow the zero mode at a point $t_1$ for which $|r_L^* r_R| = 1$, and we find that it moves away from zero for a crossover value $\Gamma_c = \beta e^{-\alpha N}$. For the specific parameters in Fig. 4, we find $\beta \simeq -8.36$ and $\alpha \simeq 0.58$ as shown in the inset of Fig. 5(f), where we have set $10^{-5}$ as the lower limit to find $\Gamma_c$. Indeed, when plotting the absolute value of the energy we see that the gap closings in the bulk bands start to move when $\Gamma \gtrsim \Gamma_c$ as shown in Figs. 5(a)-(c) for an even chain in which case the Hamiltonian is given by Eq. (2) with both entries in the right bottom corner replaced with $t_2$ and Figs. 5(d)-(e) for an odd chain. We note that when $\Gamma \neq 0$, we can no longer solve the Hamiltonian in Eq. (2) exactly.

## DOMAIN WALLS

Finally, we provide quantitative details on our discussion in the main text of a system in ring geometry with two domains $\alpha$ and $\beta$. We couple the non-Hermitian SSH chain (domain $\alpha$), whose Bloch Hamiltonian is given in Eq. (8) in the main text, to a domain $\beta$ in the form of a Hermitian chain consisting of $N_\beta$ unit cells with two sublattices, $A'$ and $B'$. The Hamiltonian reads $H_{DW} = \Psi^\dagger \mathcal{H}_{DW} \Psi$ with $\Psi^\dagger = (c_{A,1}^\dagger, c_{B,1}^\dagger, \ldots, c_{A,N_\alpha}^\dagger, c_{B,N_\alpha}^\dagger\ c_{A',1}^\dagger, c_{B',1}^\dagger, \ldots, c_{A',N_\beta}^\dagger, c_{B,N_\beta}^\dagger)$ and

$$\mathcal{H}_{DW} = \begin{pmatrix} \mathcal{H}_\alpha & \mathcal{H}_{\alpha-\beta} \\ \mathcal{H}_{\alpha-\beta}^\dagger & \mathcal{H}_\beta \end{pmatrix}, \tag{3}$$

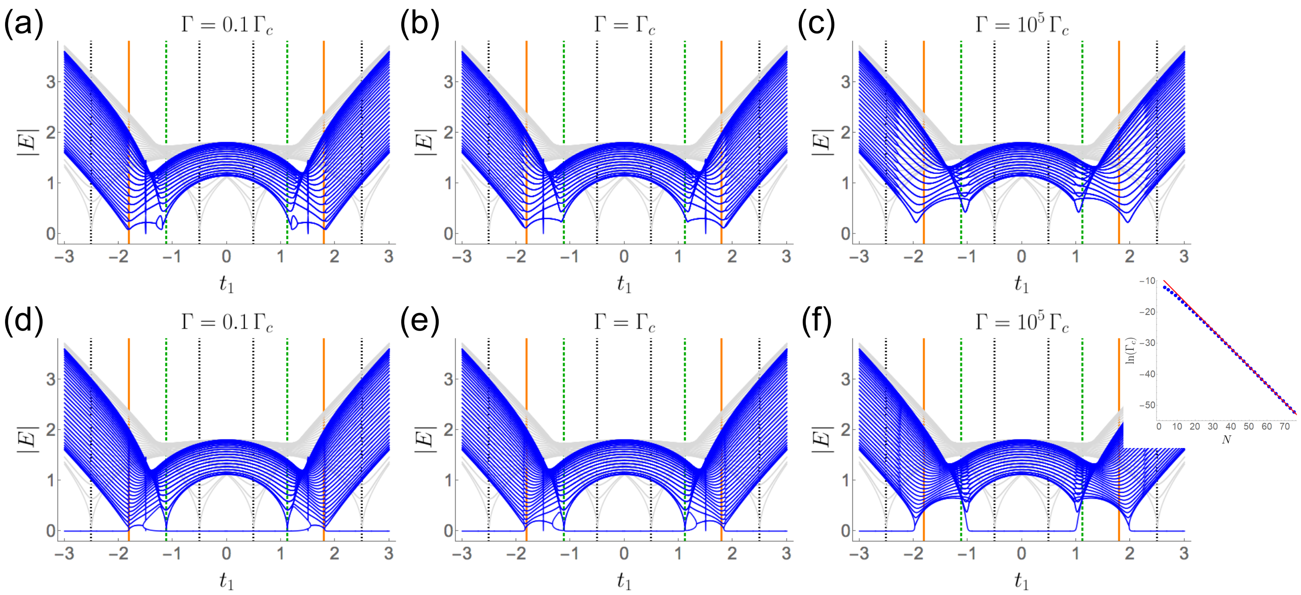


FIG. 5: The absolute value of the energy spectrum of the non-Hermitian SSH chain with chain length (a)-(c) $N = 72$ and (d)-(f) $N = 71$, and different values for $\Gamma$; (a) and (d) $\Gamma = 0.1\,\Gamma_c$, (b) and (e) $\Gamma = \Gamma_c$, and (c) and (f) $\Gamma = 10^5\,\Gamma_c$. The same parameters are used as in Fig. 4. The gray spectrum corresponds to the periodic case, and the orange (dark green dashed) vertical lines indicate those values of $t_1$ where $r_L^* r_R = 1$ ($r_L^* r_R = -1$) and the black dotted-dashed lines correspond to the EPs of the periodic Hamiltonian. The inset in (f) shows the natural logarithm of $\Gamma_c$ in blue for which the zero mode in the spectrum shown in Fig. 4 moves away from zero energy at a point $t_1$ for which $|r_L^* r_R| = 1$. The red line has a slope of $\alpha \approx 0.58$.

where

$$\mathcal{H}_\alpha = \begin{pmatrix} 0 & t_1 + \frac{\gamma}{2} & 0 & 0 & 0 \\ t_1 - \frac{\gamma}{2} & 0 & t_2 & 0 & 0 \\ 0 & t_2 & 0 & t_1 + \frac{\gamma}{2} & 0 \\ 0 & 0 & t_1 - \frac{\gamma}{2} & 0 & \cdots \\ 0 & 0 & 0 & \vdots & \ddots \end{pmatrix}, \qquad \mathcal{H}_\beta = \begin{pmatrix} 0 & t_3 & 0 & 0 & 0 \\ t_3 & 0 & t_4 & 0 & 0 \\ 0 & t_4 & 0 & \cdots & 0 \\ 0 & 0 & \vdots & \ddots & t_3 \\ 0 & 0 & 0 & t_3 & 0 \end{pmatrix}, \qquad \mathcal{H}_{\alpha-\beta} = \begin{pmatrix} 0 & 0 & 0 & \cdots & t_4 \\ 0 & 0 & 0 & \cdots & 0 \\ 0 & 0 & 0 & \cdots & 0 \\ \vdots & \vdots & \vdots & \ddots & 0 \\ t_4 & 0 & 0 & 0 & 0 \end{pmatrix}. \quad (4)$$

In Figs. 6(a)-(c) and (d)-(f), we show the absolute value of the band spectrum for a system where the non-Hermitian chains are even and odd, respectively, while the Hermitian chain is of even length in both cases. In Figs. 6(a) and (d), the spectrum of $\mathcal{H}_\beta$ has a large gap, such that the zero mode(s) of the non-Hermitian chain cannot leak into the Hermitian chain and open physics is retrieved. As discussed in the main text, when the gap becomes sufficiently small, the exponential tail of the zero mode is long enough for the mode to tunnel through the Hermitian chain, and the zero-energy band starts to move away from the EPs of the open system as shown in Figs. 6(b) and (e). As expected, the change in the spectrum for the even non-Hermitian SSH chain in (b) is more pronounced than that of the odd chain in (d) because there are two zero modes at each end, which interfere with each other. By closing the gap in the Hermitian chain further, the zero mode(s) will interfere more strongly until the spectrum is completely gapless, in which case the mode(s) can tunnel through and periodic physics is retrieved as clearly shown in Figs. 6(c) and (f).

[1] F. D. M. Haldane, *Model for a Quantum Hall Effect without Landau Levels: Condensed-Matter Realization of the "Parity Anomaly"*, Phys. Rev. Lett. **61**, 2015 (1988).
[2] Y. Xiong, *Why does bulk boundary correspondence fail in some non-hermitian topological models*, arXiv:1705.06039 (2017).

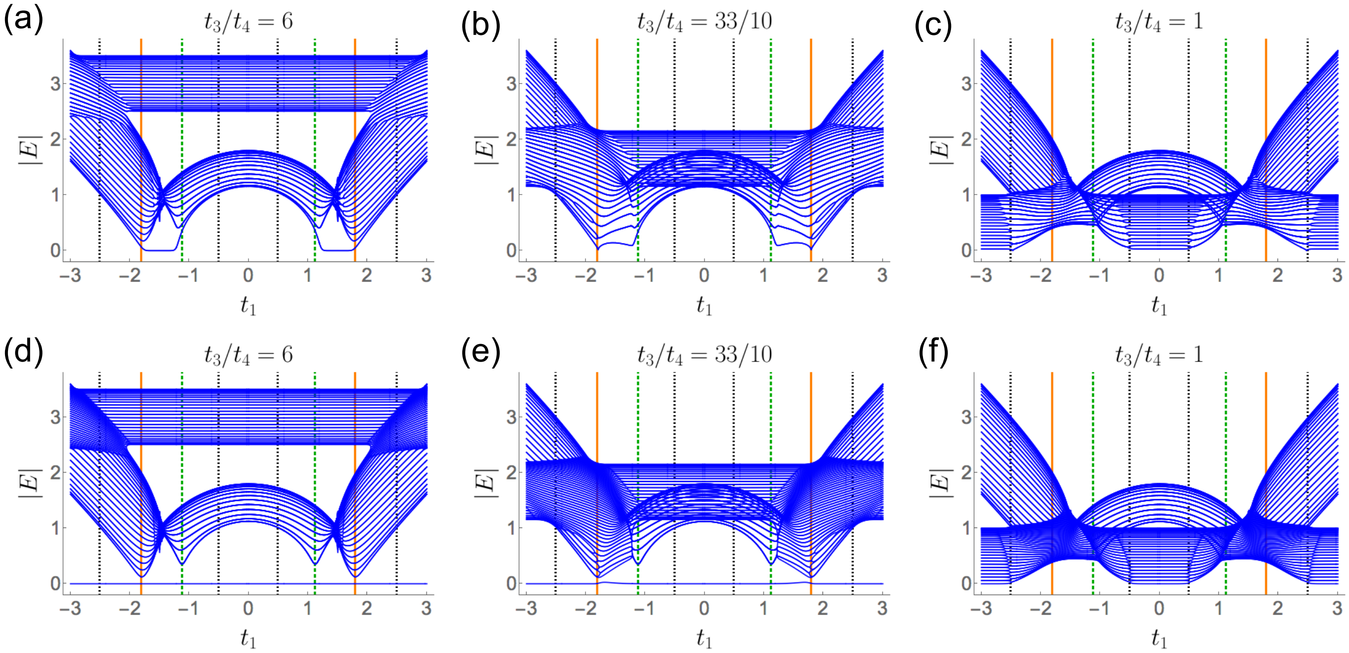


FIG. 6: The band spectrum of the Hamiltonian in Eqs. (3) and (4) with the Hermitian chain with $N_\beta = 25$ sites and the non-Hermitian chains with $N_\alpha = 25$ (a)-(c) with no broken unit cells and (d)-(f) a broken unit cell at $n_\alpha = 25$. The same parameters are used as in Fig. 4. The orange (dark green dashed) vertical lines correspond to those value of $t_1$ where $r_L^* r_R = 1$ ($r_L^* r_R = -1$) and the black dotted-dashed lines correspond to the values of $t_1$ where the Bloch Hamiltonian has EPs. The spectrum of $\mathcal{H}_\alpha$ has a large gap in (a) and (c), such that open physics is observed, whereas for a sufficiently small gap in (b) and (d) the zero mode starts to move into the Hermitian chain until periodic physics is obtained for a gapless system in (c) and (f).
